# Supplementary material for: ENInst: Enhancing Weakly-supervised Low-shot Instance Segmentation
Source: arXiv:2302.09765 source file (2023-07-31)
Supplement: Supplementary file 1 [file A.details.tex]

In this section, we explain the details, including datasets, models, ground-truth allocation algorithms, Instance-wise Mask Refinement (IMR) for mask quality enhancement, and tuned hyperparameters.
For implementation, we use PyTorch Distributed library~\cite{NEURIPS2019_bdbca288} and 2 NVIDIA GeForce RTX A6000 GPUs for base training and 1 GPU for novel fine-tuning and inference.
The code is based on Detectron2~\cite{wu2019detectron2} and AdelaiDet~\cite{tian2019adelaidet}.

\subsection{Datasets}\label{sec:A.1}
\paragraph{MS-COCO} 
MS-COCO~\cite{lin2014microsoft} is the popular visual benchmark dataset. 
To construct the low-shot version of the data split, we follow the standard low-shot data preparation~\cite{wang2020few,Ganea_2021_CVPR,fan2020fgn}.
% (this is why we constructed the COCO novel-only dataset).
The 20 classes overlapped with those of PASCAL VOC~\cite{everingham2010pascal} are used for the novel classes, and the rest 60 classes disjoint with those of PASCAL VOC are for the base classes.
The whole data in the base classes are used for pre-training.
For fine-tuning, the $K$ number of examples are randomly sampled from the novel class set and used for training.
We construct the 10 fine-tuning sub-datasets by the random sampling, and we report the average of the results over the 10 sets in all experiments to reduce the randomness in performance.

The evaluation is conducted on the standard validation set, which
we extract the 5k query images from the MS-COCO 2014 validation set.
% The rest is for \moon{pre-training on base classes and fine-tuning on novel classes;}
% % base training and novel-fine tuning; 
% the 60 classes disjoint with the classes of PASCAL VOC~\cite{everingham2010pascal} are base classes, and the rest 20 classes are novel classes.
In the cross-data setting (COCO2VOC), we use all the test data of PASCAL VOC as the query set.
% We construct the 10 fine-tuning sub-datasets and report the average of the 10 results over the sets in all experiments to reduce the randomness in performance.  
% minimize the performance errors due to randomness.

In addition, we separately construct another validation set, called the COCO novel-only dataset.
We found that the standard validation set of COCO contains many images, where no novel class objects of interest appears in those images. The amount of such a case is not negligible; thus, this may distract focusing on the novel class performance.
The COCO novel-only dataset allows to focus more on the novel class performance, rather than false positives by detection.

\paragraph{PASCAL VOC} 
PASCAL VOC~\cite{everingham2010pascal} is another popular visual benchmark dataset.
We also follow the existing low-shot related work~\cite{wang2020few,Ganea_2021_CVPR,fan2020fgn} to configure low-shot data splits.
We use the PASCAL VOC 2012 training and validation sets for constructing the pre-training and fine-tuning splits, and the test set for the query split. 
In the VOC novel test setting, we randomly split the 20 object classes into 15 base and 5 novel classes considering 3 random splits, which have the novel classes as follows: \{bird, bus, cow, motorbike, sofa\}, \{aeroplane, bottle, cow, horse, sofa\}, and \{boat, cat, motorbike, sheep, sofa\}, respectively.
We also report the average of 10 experiment results in a cross-validation manner.

\IEEEpubidadjcol
\subsection{Model}\label{sec:A.2}
We design a baseline model as an anchor-free network architecture to mitigate the anchor box biasing issue in Sec.~\ck{\rom{3}-B} of the main paper.
The baseline uses CondInst architecture~\cite{tain2020condinst} that tackles instance segmentation tasks and
% Our baseline 
contains backbone, mask branch, and prediction heads.
The backbone is composed of ResNet-50~\cite{he2016deep} and a feature pyramid network (FPN)~\cite{lin2017feature} for diverse sizes of instances in an image.
The mask branch is connected to FPN, gets features from the FPN, and is fed the features through the dynamic mask head.
The prediction heads stand for the branches of the classification, centerness, bounding box regression, and controller.
All these heads are 
% instance-specific and
constructed with a $3\times3$ convolution layer (for detail implementation of heads,
% We 
please refer to CondInst~\cite{tain2020condinst}).

The controller infers the weights of the dynamic mask head, which has three convolution layers with 169 parameters.
% The favorable property that the controller is instance-wise is proper for fast adaptation to new classes in our low-shot regime.
% \moon{The instance-wise controller is proper for fast adaptation to new classes, which is a favorable property in our low-shot regime.}
We utilize and modify the instance-wise controller part to propose an Instance-wise Mask Refinement (IMR) for mask quality enhancement.
% method,
% which can be considered as a segmentation version of MAML-like meta-learning~\cite{finn2017model}.

\newcommand{\symmask}{\mbox{\boldmath $\mathsf{m}$}}
\newcommand{\symbbox}{\mbox{\boldmath $\mathsf{b}$}}

\subsection{Ground-truth Allocation Test}\label{sec:A.3}
We propose the ground-truth allocation tests to disentangle the segmentation sub-tasks, \ie, mask quality and classification accuracy, in Sec.~\ck{\rom{4}-B} of the main paper.
We summarize our ground-truth mask allocation test in Algorithm~\ref{alg:gt_mask_alloc}.

\begin{algorithm}[t]
\SetAlgoLined
    \textbf{Input:} prediction labels $\{\Tilde{\textbf{b}}_j, \Tilde{\textbf{m}}_j\}_{j=1}^{N_\bI^p}$,\\ 
    ground-truth labels $\{\symbbox_i, \symmask_i\}_{i=1}^{N_\bI}$,\\
    $N_\bI^p$ is the number of predicted instances, and \\
    $N_\bI$ is the number of ground-truth instances in an image $\bI$\\
    \vspace{2mm}
    \For{$j=1,2,\dots,N_\bI^p$}{
        \For{$i=1,2,\dots,N_\bI$}{
             IoUs$_{ji}=$compute IoU between $\Tilde{\textbf{b}}_j$ and $\symbbox_i$\;}
        $k = \texttt{argmax}_i$ IoUs$_{ji}$\;
        $\Tilde{\textbf{m}}_j := \symmask_k$\;
    }
    \textbf{Output:} allocated ground-truth masks $\{\symmask_j\}_{j=1}^{N_\bI^p}$
    \caption{Ground-truth Mask Allocation}
    \label{alg:gt_mask_alloc}
\end{algorithm}
% \vspace{-2mm}

\begin{table}
    % \vspace{-8mm}
    \centering
    \caption{
    % Mask refinement 
    Hyperparameter settings for IMR \wrt the number of iterations and learning rate. 
    We follow the Standard setting in this table unless specified.
    % The settings that are not specified follow the Standard setting.
    We use AdamW optimizer.
    The $\mathcal{WF}$ and $\mathcal{WW}$ supervision settings are defined in \Sref{sec:B}.
    } 
    \resizebox{1.0\linewidth}{!}{\footnotesize
    \begin{tabular}{l@{\quad}c@{\quad}c} 
        \toprule
        \textbf{Test Setting} & \textbf{\# Iterations} & \textbf{Learning Rate} \\
        \midrule
            Standard & 10 & 0.05 \\
            VOC novel & 30 & 0.05 \\
            $\mathcal{WF}$ and $\mathcal{WW}$ (COCO novel-only) & 10 & 0.01\\
            % COCO novel-only $\mathcal{WF}$ & 10 & 0.01\\
            % COCO novel $\mathcal{WW}$ & 10 & 0.01\\
            % COCO novel-only $\mathcal{WW}$ & 10 & 0.01\\
        \bottomrule
    \end{tabular}
    }
    \label{tab:optimization_hyper}
\end{table}

\begin{table*}[ht!]
    \centering
    \caption{Supervision setting comparison on the COCO novel-only setting. 
    The first column represents the label types used in the pre-training and fine-tuning phases, where $\mathcal{F}$ denotes full supervision with mask, and $\mathcal{W}$ weak one with bounding box.
    \textbf{Bold} indicates the best results in each weak data setting.
    % , and \pink{brick} color represents higher performance than the fully-supervised model. 
    }
    \resizebox{\linewidth}{!}
    {\footnotesize
    \begin{tabular}{c l TTTT TTTT TTTT} 
        \toprule
        \multirow{3}[3]{*}{\textbf{Label}} & \multirow{3}[3]{*}{\textbf{Model}} & \multicolumn{4}{c}{\textbf{1-shot}} & \multicolumn{4}{c}{\textbf{5-shot}} & \multicolumn{4}{c}{\textbf{10-shot}}\\
        \cmidrule(lr){3-6} \cmidrule(lr){7-10} \cmidrule(lr){11-14}
        & & \multicolumn{2}{c}{\textbf{Detection}} & \multicolumn{2}{c}{\textbf{Segmentation}} & \multicolumn{2}{c}{\textbf{Detection}} & \multicolumn{2}{c}{\textbf{Segmentation}} & \multicolumn{2}{c}{\textbf{Detection}} & \multicolumn{2}{c}{\textbf{Segmentation}}\\
        \cmidrule(lr){3-4} \cmidrule(lr){5-6} \cmidrule(lr){7-8} \cmidrule(lr){9-10} \cmidrule(lr){11-12} \cmidrule(lr){13-14}
        & & \textbf{AP} & \textbf{AP50} & \textbf{AP} & \textbf{AP50} & \textbf{AP} & \textbf{AP50} & \textbf{AP} & \textbf{AP50} & \textbf{AP} & \textbf{AP50} & \textbf{AP} & \textbf{AP50} \\ 
        \midrule
          $\mathcal{FF}$ & MTFA 
          & 2.82 & 5.55 & 2.97 & 5.16 
          & 7.27 & 13.59 & 7.21 & 12.69 
          & 9.27 & 16.99 & 9.02 & 15.88 \\ 
        \midrule
          \multirow{3}{*}{$\mathcal{FW}$} 
          & GrabCut 
             & 2.25 &  4.15 & 0.96 & 2.15
             & 6.74 & 12.22 & 2.67 & 5.92
             & 9.28 & 16.79 & 3.51 & 7.93 \\ 
          & Baseline 
             & 2.25 &  4.15 & 2.04 &  3.66 
             & 6.74 & 12.22 & 5.93 & 10.89
             & 9.28 & 16.79 & 7.94 & 14.72 \\ 
        %   & +NCC+MMF
        %      & 2.59 & 4.89 & 2.27 & 4.17 
        %      & 7.23 & 13.04 & 6.18 & 11.55
        %      & 9.81 & 17.60 & 8.33 & 15.46 \\
        %   & +Mask Refinement 
        %      & 2.25 &  4.15 & 2.10 &  3.69 
        %      & 6.74 & 12.22 & 6.10 & 10.99
        %      & 9.28 & 16.79 & 8.17 & 14.88 \\ 
          & ENInst (Ours)
             & \textbf{2.59} & \textbf{ 4.89} & \textbf{2.34} & \textbf{ 4.18}
             & \textbf{7.23} & \textbf{13.04} & \textbf{6.35} & \textbf{11.65}
             & \textbf{9.81} & \textbf{17.60} & \textbf{8.54} & \textbf{15.57}\\ 
        \midrule                
          \multirow{3}{*}{$\mathcal{WF}$}
          & GrabCut 
             & 1.90 &  3.49 & 0.76 & 1.75
             & 5.96 & 10.78 & 2.42 & 5.44
             & 8.55 & 15.58 & 3.24 & 7.34 \\
          & Baseline 
             & 1.90 &  3.49 & 1.59 &  3.06 
             & 5.96 & 10.78 & 5.11 &  9.55
             & 8.55 & 15.58 & \textbf{7.36} & \textbf{13.93} \\ 
        %   & +NCC+MMF
        %      & 2.16 &  4.07 & 1.77 &  3.54 
        %      & 6.70 & 12.11 & 5.54 & 10.62 
        %      & 8.75 & 15.82 & 7.26 & 13.99 \\
        %   & +Mask Refinement
        %      & 1.90 &  3.49 & & 
        %      & 5.96 & 10.78 & & 
        %      & 8.55 & 15.58 & & \\
          & ENInst-$\mathcal{WF}$
             & \textbf{2.16} & \textbf{ 4.07} & \textbf{1.70} & \textbf{ 3.47} 
             & \textbf{6.70} & \textbf{12.11} & \textbf{5.27} & \textbf{10.34} 
             & \textbf{8.75} & \textbf{15.82} & 6.90 & 13.58 \\
        \midrule                   
          \multirow{3}{*}{$\mathcal{WW}$}
          & GrabCut 
             & 1.94 &  3.55 & 0.75 & 1.75 
             & 5.82 & 10.43 & 2.38 & 5.29
             & 8.18 & 15.03 & 3.06 & 6.91 \\ 
          & Baseline 
             & 1.94 &  3.55 & 1.54 &  2.98 
             & 5.82 & 10.43 & 4.69 &  8.94 
             & 8.18 & 15.03 & 6.42 & 12.66 \\ 
        %   & +NCC+MMF 
        %      & 2.11 &  3.92 & 1.71 &  3.34 
        %      & 6.50 & 11.71 & 5.08 &  9.91 
        %      & 8.86 & 15.95 & 6.79 & 13.43 \\
        %   & +Mask Refinement
        %      & 1.94 &  3.55 & 1.54 &  2.99 
        %      & 5.82 & 10.43 & 4.70 &  8.96 
        %      & 8.18 & 15.03 & 6.46 & 12.71 \\
          & ENInst-$\mathcal{WW}$
             & \textbf{2.11} & \textbf{ 3.92} & \textbf{1.71} & \textbf{ 3.32} 
             & \textbf{6.50} & \textbf{11.71} & \textbf{5.10} & \textbf{ 9.93} 
             & \textbf{8.86} & \textbf{15.95} & \textbf{6.83} & \textbf{13.44} \\
        \bottomrule
    \end{tabular}
    }
    \label{tab:baseline_comparison}
    % \vspace{-1mm}
\end{table*}

With these variables, we optimize the dynamic mask head and refine the instance-wise mask prediction.
The optimization hyperparameters, \ie, the number of iterations and learning rate, may change depending on the test settings. 
We use the hyperparameters in \Tref{tab:optimization_hyper}.
We use different iterations in the VOC novel test setting and different learning rates in 
different supervision settings explained in \Sref{sec:B}.

% \subsection{Instance-wise Mask Refinement}\label{sec:A.4}
% iterative results
% \begin{figure*}[t!]
%      \centering
%      \includegraphics[width=1.0\linewidth]{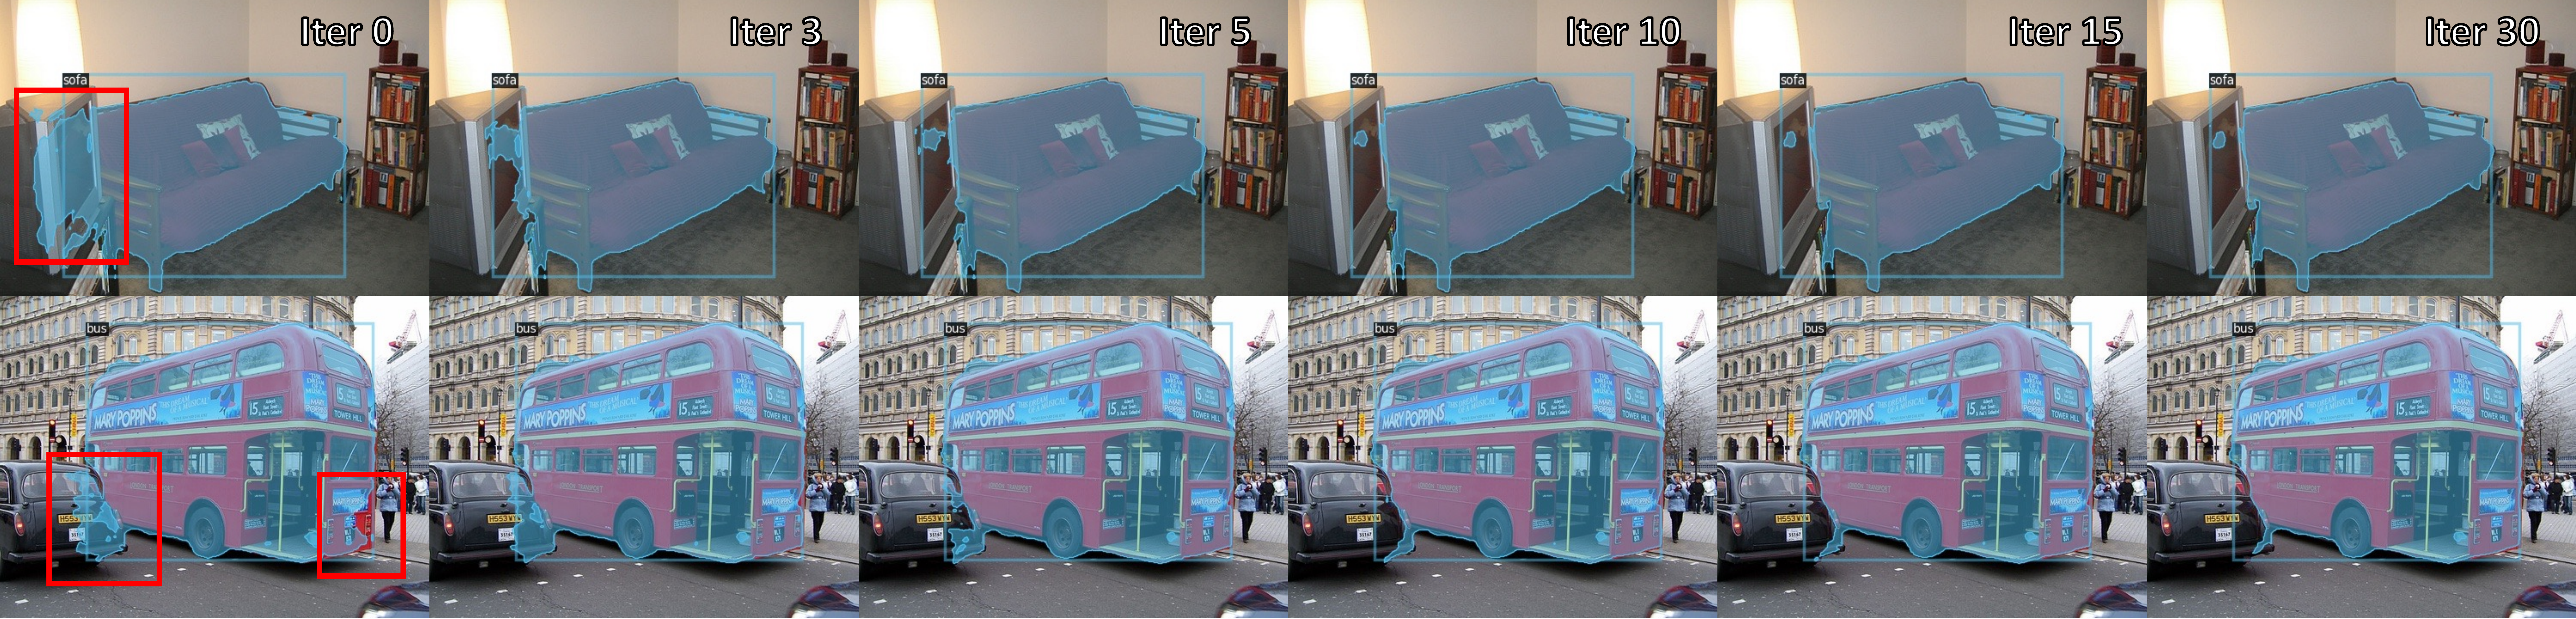}   
%      \caption{IMR iter.}
%      \label{fig:imr_iter}
% \end{figure*}

\subsection{Novel Classifier Composition}\label{sec:A.4}
The visualization of the full weights $\balpha'\in\mathbb{R}^{|\cbase|\times |\cnovel|}$ in \Fref{fig:ncc_vis_full} shows the correlation between base and novel classes in MS-COCO.
The full version result also shows the similar tendency with Fig.~\ck{7} in the main paper, which implies that the prior knowledge of base classes is of use to represent the novel classes.
\begin{figure}[h!]
    \centering
    \includegraphics[width=1.0\linewidth]{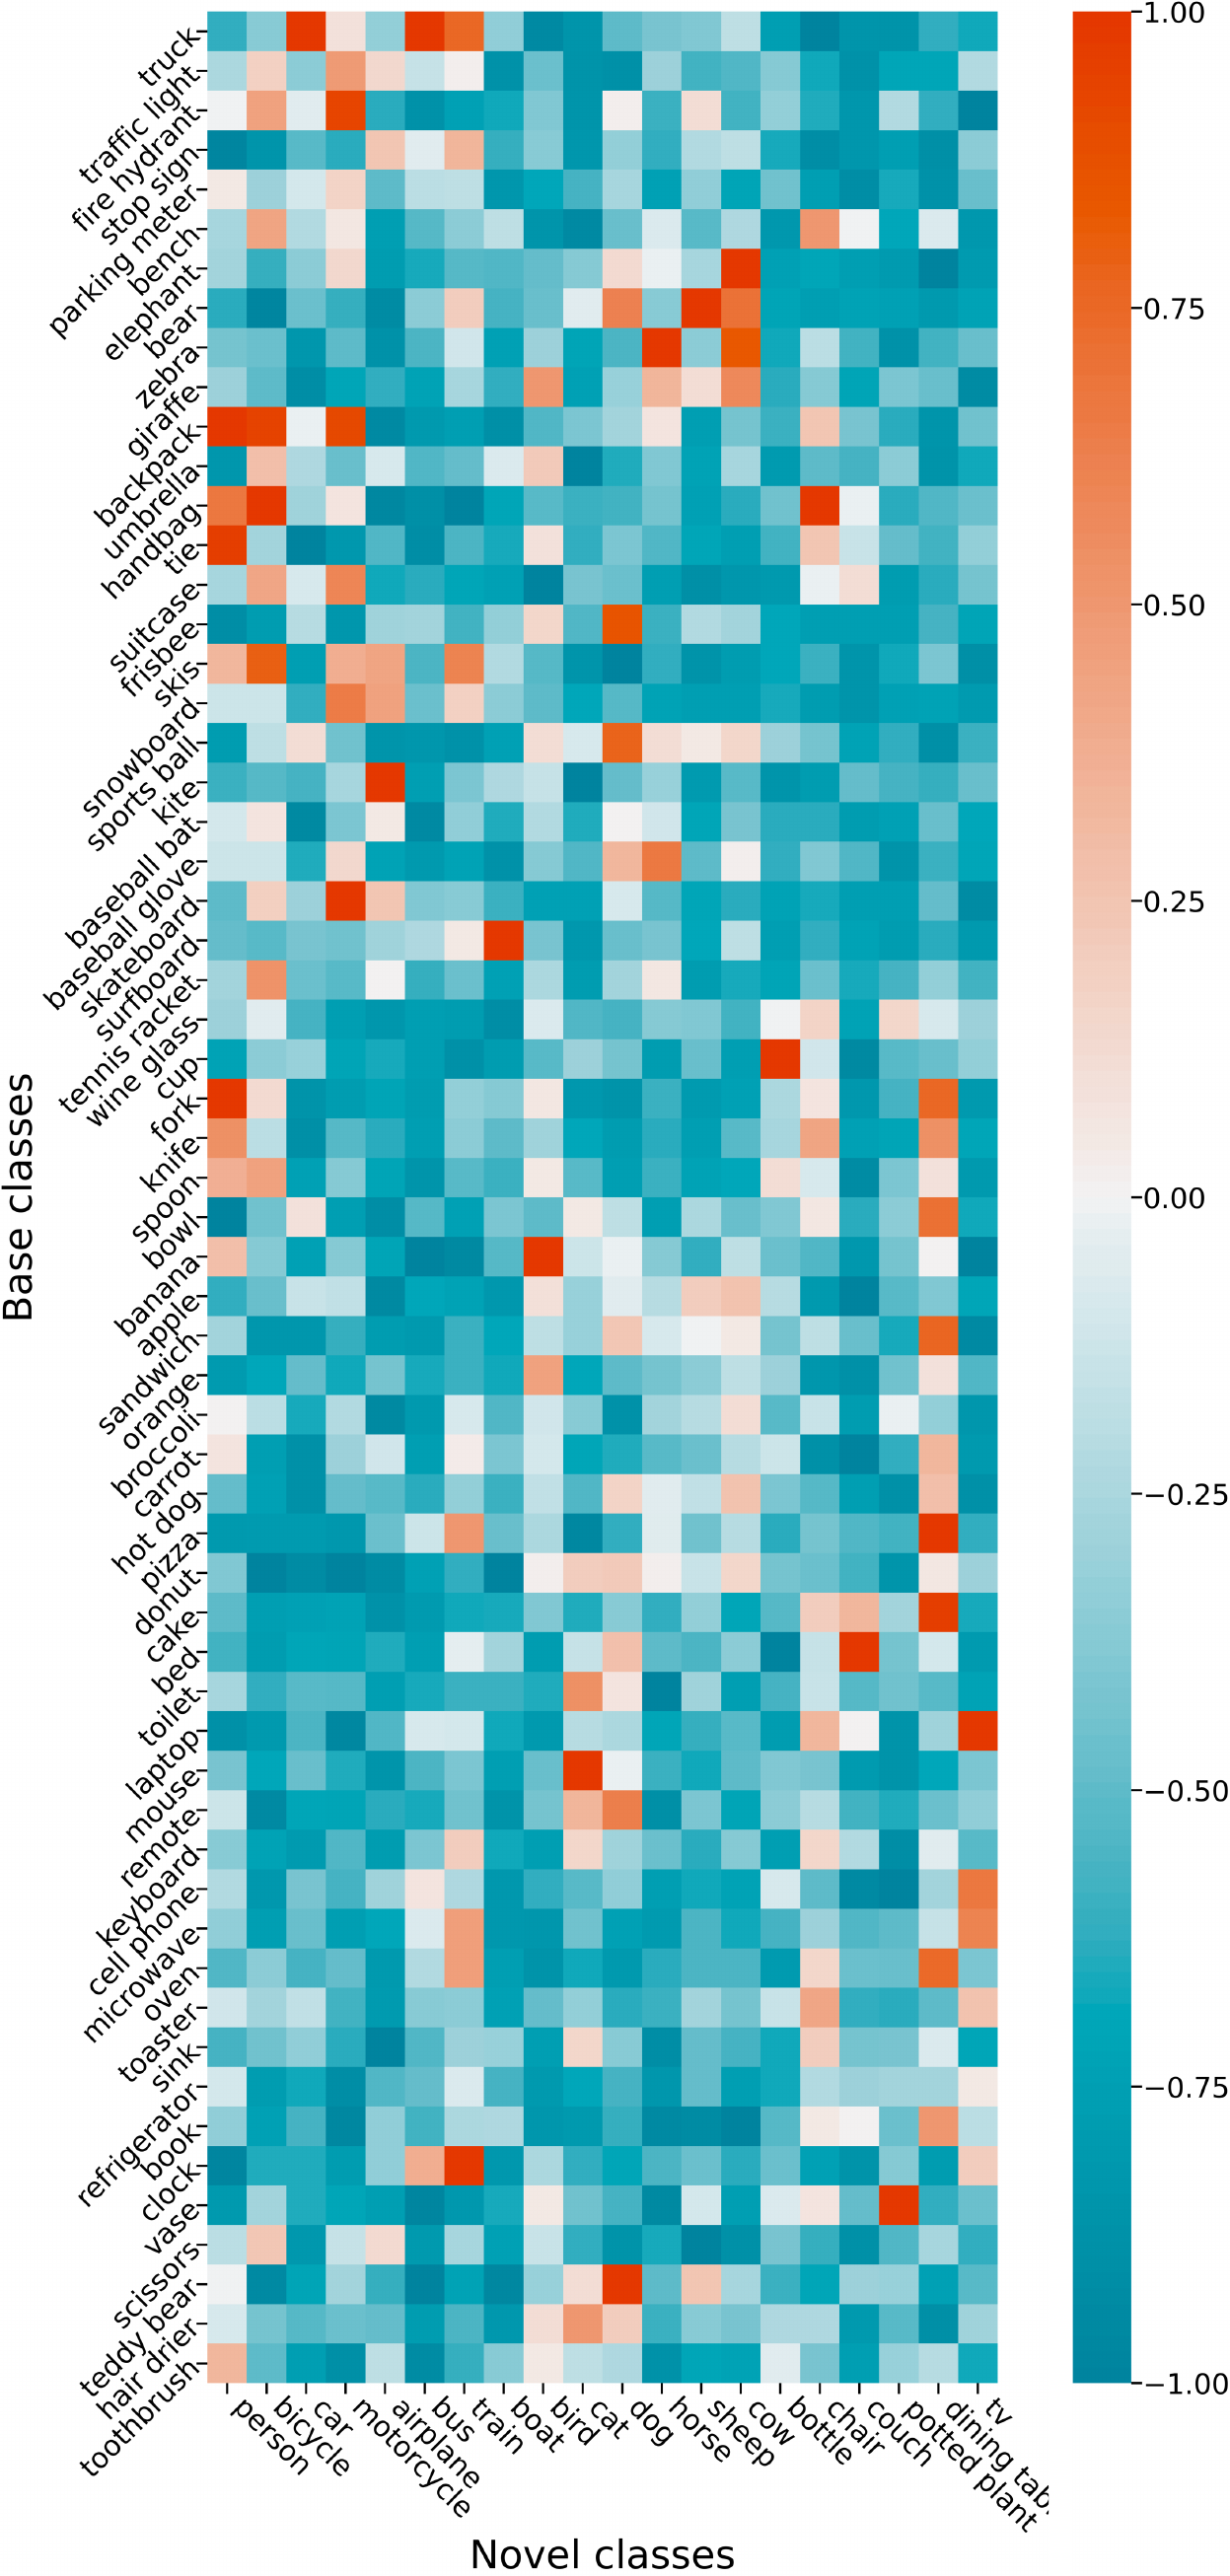}
    \caption{Visualization of the full weights in NCC, \ie, correlation between base and novel classes in MS-COCO. 
    Red color stands for high correlation and blue color for low correlation.}
    \label{fig:ncc_vis_full}
\end{figure}

\subsection{Hyperparameters}\label{sec:A.5}
We explain hyperparameters and more details about the pre-training phase for learning base classes and fine-tuning phase for learning novel classes, \wrt batch size, learning rate, the number of iterations, and scheduler.
In the pre-training phase, we train the whole network by SGD with batch size 8, 0.01 learning rate, 90,000 iterations for COCO and 20,000 for VOC, and 0.9 momentum.

In the fine-tuning phase, we train the prediction heads by SGD with batch size 8 and 0.005 learning rate. 
The number of iterations is different for each shot setting.
On MS-COCO, we set 500 iterations for 1-shot, 500 for 5-shot, 800 for 10-shot, and 1,000 for 30-shot.
On PASCAL VOC, we set 100 iterations for 1-shot, 500 for 5-shot and 10-shot.
The study on the effect of iterations is separately addressed in Sec.~\ref{sec:C.2}.
