# Supplementary material for: ENInst: Enhancing Weakly-supervised Low-shot Instance Segmentation
Source: arXiv:2302.09765 source file (2023-07-31)
Supplement: Supplementary file 2 [file B.comparison.tex]

The original weakly-supervised setting for LSIS employs full supervision in the pre-training phase and weak supervision in the fine-tuning phase, \ie, full-weak~($\mathcal{FW}$) setting.
The $\mathcal{FW}$ setting can strongly train the feature extractor part with full supervision.
It only needs a handful number of box annotations for the novel classes, which is favorable when deploying in practice.

Besides, our model architecture and methods are compatible with different supervision settings at each phase, such as weak-full~($\mathcal{WF}$) and weak-weak~($\mathcal{WW}$) settings.
We anticipate that both $\mathcal{WF}$ and $\mathcal{WW}$ settings have a relatively weak feature extractor and performance degradation, but these settings still have their own good trade-offs.

Therefore, we conduct the performance comparison of the baseline and our ENInst on all the possible weakly-supervised data settings for low-shot instance segmentation: $\mathcal{FW}$, $\mathcal{WF}$ and $\mathcal{WW}$ settings.
In Table \ref{tab:baseline_comparison}, we denote ENInst on the original setting as ENInst (Ours), and on $\mathcal{WF}$ and $\mathcal{WW}$ as ENInst-$\mathcal{WF}$ and ENInst-$\mathcal{WW}$, respectively.
ENInst-$\mathcal{WF}$ and ENInst-$\mathcal{WW}$ are trained as the same as ENInst (Ours) except for the mask prediction loss functions in each phase.

\paragraph{Dataset}
To compare the possible weakly-supervised settings for low-shot instance segmentation, we follow the standard few- and low-shot split~\cite{fan2020fgn,Ganea_2021_CVPR,wang2020few} with MS-COCO~\cite{lin2014microsoft} as mentioned in \Sref{sec:A.1}.
To suppress the effects of false positives and focus more on the supervision setting comparison, we use the COCO novel-only setting, as in Sec.~\ck{\rom{4}} of the main paper.

\paragraph{Comparison}
We compare all the possible weakly settings on the baseline and ENInst in Table \ref{tab:baseline_comparison}.
Due to the lack of competing methods handling the same tasks, we construct another strong baseline based on GrabCut~\cite{Rother2004GrabCutIF} in each setting and compare it within all the supervision settings.
We also compare with MTFA~\cite{Ganea_2021_CVPR}, which is the fully-supervised few-shot instance segmentation, for reference.

\begin{table*}[ht!]
    % \vspace{-3mm}
    \centering
    \caption{Comparison on the COCO novel setting (Full version of Fig.~\ck{1} in the main paper).
    The first column represents the label type used in the fine-tuning phase, where $\mathcal{F}$ denotes full supervision with mask, and $\mathcal{W}$ weak one with bounding box.
    \textbf{Bold} indicates the best results in original weak data setting, \ie, $\mathcal{FW}$ setting.
    % The configuration follows \Tref{tab:baseline_comparison}.
    % \textbf{Bold} indicates the best results in \moon{$\mathcal{FW}$ setting.}
    % each weak data setting
    % , and the \pink{brick} color represents higher performance than the most elevated fully-supervised model. 
    }  
    \resizebox{\linewidth}{!}
    {\footnotesize
    \begin{tabular}{c l TTTT TTTT TTTT TTTT} 
        \toprule
        \multirow{3}[3]{*}{\textbf{Label}} & \multirow{3}[3]{*}{\textbf{Model}} & \multicolumn{4}{c}{\textbf{1-shot}} & \multicolumn{4}{c}{\textbf{5-shot}} & \multicolumn{4}{c}{\textbf{10-shot}} & \multicolumn{4}{c}{\textbf{30-shot}}\\
        \cmidrule(lr){3-6} \cmidrule(lr){7-10} \cmidrule(lr){11-14} \cmidrule(lr){15-18}
        & & \multicolumn{2}{c}{\textbf{Detection}} & \multicolumn{2}{c}{\textbf{Segmentation}} & \multicolumn{2}{c}{\textbf{Detection}} & \multicolumn{2}{c}{\textbf{Segmentation}} & \multicolumn{2}{c}{\textbf{Detection}} & \multicolumn{2}{c}{\textbf{Segmentation}} & \multicolumn{2}{c}{\textbf{Detection}} & \multicolumn{2}{c}{\textbf{Segmentation}}\\
        \cmidrule(lr){3-4} \cmidrule(lr){5-6} \cmidrule(lr){7-8} \cmidrule(lr){9-10} \cmidrule(lr){11-12} \cmidrule(lr){13-14} \cmidrule(lr){15-16} \cmidrule(lr){17-18}
        & & \textbf{AP} & \textbf{AP50} & \textbf{AP} & \textbf{AP50} & \textbf{AP} & \textbf{AP50} & \textbf{AP} & \textbf{AP50} & \textbf{AP} & \textbf{AP50} & \textbf{AP} & \textbf{AP50} & \textbf{AP} & \textbf{AP50} & \textbf{AP} & \textbf{AP50} \\ 
        \midrule
           \multirow{3}{*}{$\mathcal{F}$} 
           & MRCN+ft-full
             &  -  &  -  &  -  &  -
             & 1.3 & 3.0 & 1.3 & 2.7
             & 2.5 & 5.7 & 1.9 & 4.7 
             & *4.5 & *9.8 & *3.7 & *8.5 \\
           & Meta R-CNN
             &  -  &   -  &  -  &   -
             & 3.5 &  9.9 & 2.8 &  6.9
             & 5.6 & 14.2 & 4.4 & 10.6 
             & *6.2 & *16.6 & *6.4 & *14.8 \\
           & MTFA 
             &  2.47 &  4.85 &  2.66 &  4.56 
             &  6.61 & 12.32 &  6.62 & 11.58
             &  8.52 & 15.53 &  8.39 & 14.64 
             & 10.71 & 19.17 & 10.32 & 18.06 \\ 
        \midrule
           \multirow{3}{*}{$\mathcal{W}$} 
           & GrabCut 
             &  2.00 &  3.69 & 0.87 & 1.93
             &  6.19 & 11.19 & 2.50 & 5.54
             &  8.58 & 15.50 & 3.31 & 7.42 
             & 11.24 & 20.20 & 3.96 & 8.85 \\
           & Baseline 
             &  2.00 &  3.69 & 1.81 &  3.26
             &  6.19 & 11.19 & 5.49 & 10.01
             &  8.58 & 15.50 & 7.40 & 13.64 
             & 11.24 & 20.20 & 9.76 & 18.07 \\
        %   & +NCC+MMF
        %      & 2.25 & 4.26 & 2.00 & 3.65 
        %      & 6.56 & 11.79 & 5.65 & 10.50
        %      & 8.97 & 16.05 & 7.70 & 14.19 \\
        %   & +Mask Refinement 
        %      & 2.00 &  3.69 & 1.87 &  3.28 
        %      & 6.19 & 11.19 & 5.65 & 10.11 
        %      & 8.58 & 15.50 & 7.61 & 13.79 \\
           & ENInst (Ours)
             & \textbf{ 2.25} & \textbf{ 4.26} & \textbf{ 2.06} & \textbf{ 3.66} 
             & \textbf{ 6.56} & \textbf{11.79} & \textbf{ 5.78} & \textbf{10.57}
             & \textbf{ 8.97} & \textbf{16.05} & \textbf{ 7.89} & \textbf{14.29} 
             & \textbf{11.43} & \textbf{20.74} & \textbf{10.07} & \textbf{18.52} \\ 
        \bottomrule
        \addlinespace[1mm]
        \multicolumn{18}{r}{*20-shot results}
    \end{tabular}
    }
    \label{tab:coco_novel_}
\end{table*}

\begin{table*}[t]
\centering
\caption{Comparison on the VOC novel setting (Full version of Table \ck{\rom{5}} in the main paper). 
% The configuration follows \Tref{tab:coco_novel_}.
The second column represents the label type used in the fine-tuning phase, where $\mathcal{F}$ denotes full supervision with mask, and $\mathcal{W}$ weak one with bounding box.
\textbf{Bold} indicates the best results in the original weak supervision setting, \ie, $\mathcal{FW}$ setting, and the \pink{brick} color represents higher performance than the fully-supervised model.
}
\resizebox{1.0\linewidth}{!}{
% \footnotesize
    \begin{tabular}{c@{\quad}c@{\quad} l@{\ } TTTT TTTT TTTT} 
        \toprule
        \multirow{3}[3]{*}{\textbf{Shots}} & \multirow{3}[3]{*}{\textbf{Label}}  & \multirow{3}[3]{*}{\textbf{Method}} 
        & \multicolumn{4}{c}{\textbf{Novel Class Setup 1}} & \multicolumn{4}{c}{\textbf{Novel Class Setup 2}} 
        & \multicolumn{4}{c}{\textbf{\textbf{Novel Class Setup 3}}} \\ 
        \cmidrule(lr){4-7} \cmidrule(lr){8-11} \cmidrule(lr){12-15}
        & & & \multicolumn{2}{c}{\textbf{Detection}} & \multicolumn{2}{c}{\textbf{Segmentation}} &
            \multicolumn{2}{c}{\textbf{Detection}} & \multicolumn{2}{c}{\textbf{Segmentation}} & \multicolumn{2}{c}{\textbf{Detection}} & \multicolumn{2}{c}{\textbf{Segmentation}}  \\ 
        \cmidrule(lr){4-5} \cmidrule(lr){6-7} \cmidrule(lr){8-9} \cmidrule(lr){10-11} \cmidrule(lr){12-13} \cmidrule(lr){14-15}
        & & & \textbf{AP} & \textbf{AP50} & \textbf{AP} & \textbf{AP50} & \textbf{AP} & \textbf{AP50} 
          & \textbf{AP} & \textbf{AP50} & \textbf{AP} & \textbf{AP50} & \textbf{AP} & \textbf{AP50} \\ 
        \midrule
        \multirow{4}[4]{*}{$K$=1} 
        & $\mathcal{F}$
        & MTFA     & 11.40 & 30.80 & 12.79 & 28.42 
                   &  7.08 & 19.75 &  7.74 & 17.74 
                   & 10.88 & 26.01 &  9.42 & 21.88 \\ 
        \cmidrule(lr){2-15}  
        & \multirow{3}{*}{$\mathcal{W}$} 
        & GrabCut  &  9.42 & 18.42 &  4.16 &  9.25 
                   &  4.59 & 10.92 &  2.83 &  6.72 
                   &  5.14 & 11.28 &  1.82 &  4.43 \\ 
        & & Baseline &  9.42 & 18.42 &  8.27 & 16.66 
                   &  4.59 & 10.92 &  4.55 &  9.78 
                   &  5.14 & 11.28 &  3.34 &  8.51 \\
        % & & +NCC+MMF  & 14.11 & 27.37 & 12.48 & \textbf{24.40}
        %           &  7.74 & 17.58 &  6.98 & \textbf{15.25}
        %           &  9.29 & 20.42 &  6.62 & 16.28 \\ 
        % & & +Mask Refinement     &  9.42 & 18.42 &  8.48 & 16.56 
        %           &  4.59 & 10.92 &  4.84 &  9.88
        %           &  5.14 & 11.28 &  3.65 &  8.97 \\
        & & ENInst (Ours)
                   & \textbf{\pink{14.11}} & \textbf{27.37} & \textbf{12.52} & \textbf{24.29}
                   & \textbf{\pink{ 7.74}} & \textbf{17.58} & \textbf{ 7.27} & \textbf{15.08}
                   & \textbf{ 9.29} & \textbf{20.42} & \textbf{ 7.34} & \textbf{16.77} \\
        \midrule
        \multirow{4}[4]{*}{$K$=5}
        & $\mathcal{F}$
        & MTFA     & 21.37 & 50.66 & 21.66 & 45.14 
                   & 13.06 & 32.85 & 11.52 & 27.16 
                   & 19.97 & 46.25 & 16.87 & 38.57 \\ 
        \cmidrule(lr){2-15}
        & \multirow{3}{*}{$\mathcal{W}$}
        & GrabCut  & 16.96 & 31.82 &  6.56 & 15.02 
                   & 11.04 & 23.46 &  6.01 & 13.50 
                   & 12.83 & 26.17 &  4.87 & 11.51 \\ 
        & & Baseline & 16.96 & 31.82 & 13.42 & 26.43 
                   & 11.04 & 23.46 &  9.07 & 19.42 
                   & 12.83 & 26.17 &  7.83 & 19.53 \\
        % & & +NCC+MMF & 20.75 & 38.95 & 16.58 & \textbf{32.54}
        %           & 15.16 & 31.13 & 11.86 & \textbf{25.14}
        %           & 16.87 & 34.63 & 10.83 & 26.43 \\ 
        % & & +Mask Refinement    & 16.96 & 31.82 & 13.95 & 26.71 
        %           & 11.04 & 23.46 &  9.59 & 19.62 
        %           & 12.83 & 26.17 &  8.38 & 20.00 \\
        & & ENInst (Ours)
                   & \textbf{20.75} & \textbf{38.95} & \textbf{16.81} & \textbf{32.42}
                   & \textbf{\pink{15.16}} & \textbf{31.13} & \textbf{\pink{12.45}} & \textbf{25.02}
                   & \textbf{16.87} & \textbf{34.63} & \textbf{11.91} & \textbf{27.46} \\
        \midrule
        \multirow{4}[4]{*}{$K$=10}
        & $\mathcal{F}$
        & MTFA     & 24.72 & 56.94 & 24.76 & 50.82 
                   & 15.26 & 32.78 & 13.30 & 30.57 
                   & 21.91 & 49.89 & 18.10 & 41.32 \\ 
        \cmidrule(lr){2-15}
        & \multirow{3}{*}{$\mathcal{W}$}
        & GrabCut  & 22.54 & 40.93 &  8.57 & 19.09 
                   & 14.82 & 29.58 &  7.47 & 16.93 
                   & 18.08 & 35.89 &  6.82 & 15.76 \\ 
        & & Baseline & 22.54 & 40.93 & 17.42 & 34.15 
                   & 14.82 & 29.58 & 11.93 & 24.90 
                   & 18.08 & 35.89 & 11.44 & 27.76 \\
        % & & +NCC+MMF  & 26.70 & 48.14 & 21.62 & 40.93
        %           & 18.50 & 36.10 & 14.43 & 29.83 
        %           & 21.38 & 42.63 & 13.94 & 33.13 \\ 
        % & & +Mask Refinement     & 22.54 & 40.93 & 17.84 & 34.47 
        %           & 14.82 & 29.58 & 12.39 & 25.15 
        %           & 18.08 & 35.89 & 12.12 & 28.07 \\
        & & ENInst (Ours)
                   & \textbf{\pink{26.70}} & \textbf{48.14} & \textbf{21.80} & \textbf{40.65} 
                   & \textbf{\pink{18.50}} & \textbf{\pink{36.10}} & \textbf{\pink{14.89}} & \textbf{29.74}
                   & \textbf{21.38} & \textbf{42.63} & \textbf{15.10} & \textbf{33.89} \\ 
        \bottomrule
    \end{tabular}
}
    \label{tab:voc2voc_}
    % \vspace{-2mm}
\end{table*}

The results show that the baseline performance on the original setting ($\mathcal{FW}$ setting) is highest among the weak supervision settings, as we postulated.
Despite the difference between the settings, the performance of the baseline is about twice as high as the GrabCut counterpart.
Surprisingly, our ENInst in the original weak setting achieves comparable performance with the fully-supervised MTFA and even surpasses the MTFA in the 10-shot detection performance in the $\mathcal{FW}$ setting.
EnInst in $\mathcal{WF}$ and $\mathcal{WW}$ settings also outperform the baseline in each setting except for 10-shot segmentation performance in $\mathcal{WF}$ setting.
The results suggest that our enhancement methods can help regardless of settings.
In short, we confirm that there is a trade-off between annotation efficiency and performance, implying that which supervision is used in each phase affects the trade-off a lot.
We suppose that $\mathcal{FW}$ setting is a good representative trade-off between performance and label efficiency for novel classes.
