# Supplementary material for: ENInst: Enhancing Weakly-supervised Low-shot Instance Segmentation
Source: arXiv:2302.09765 source file (2023-07-31)
Supplement: Supplementary file 3 [file C.add_exp.tex]

We report the full versions of the experiment tables or graph figure in the main paper and additional experiments in \Sref{sec:C.1}. 
We also conduct the iteration test to observe the effects of fine-tuning in \Sref{sec:C.2}.

\subsection{Additional Results of ENInst}\label{sec:C.1}
\paragraph{COCO Novel}
We report the full version of Fig.~\ck{1} presented in the main paper and additionally evaluate our method on the COCO novel setting in \Tref{tab:coco_novel_}.
The results consist of 1, 5, 10, 30 shot cases.
On all the settings, the baseline performs about twice better than the weakly-supervised GrabCut counterpart in segmentation.
The baseline also shows better segmentation performance than the two fully-supervised models, MRCN+ft-full and Meta R-CNN.
Although the baseline has lower performance than fully-supervised MTFA, our ENInst bridge the performance gap considerably, demonstrating that our enhancement methods, IMR and NCC, can effectively fill the insufficient information of weak labels.
In addition, the results show that as the number of shots increases, so does the efficiency of our method.

We show additional qualitative results of our ENInst on the MS-COCO dataset~\cite{lin2014microsoft} in \Fref{fig:qualitative_coco_novel}.
There are 20 classes and diverse sizes of instances and images in the query dataset.
Despite the change in size and visible part of the instance, we show qualitative results for various classes with only 10 number of weakly-labeled examples.

\begin{figure*}[t]
    \centering
    \includegraphics[width=1.0\linewidth]{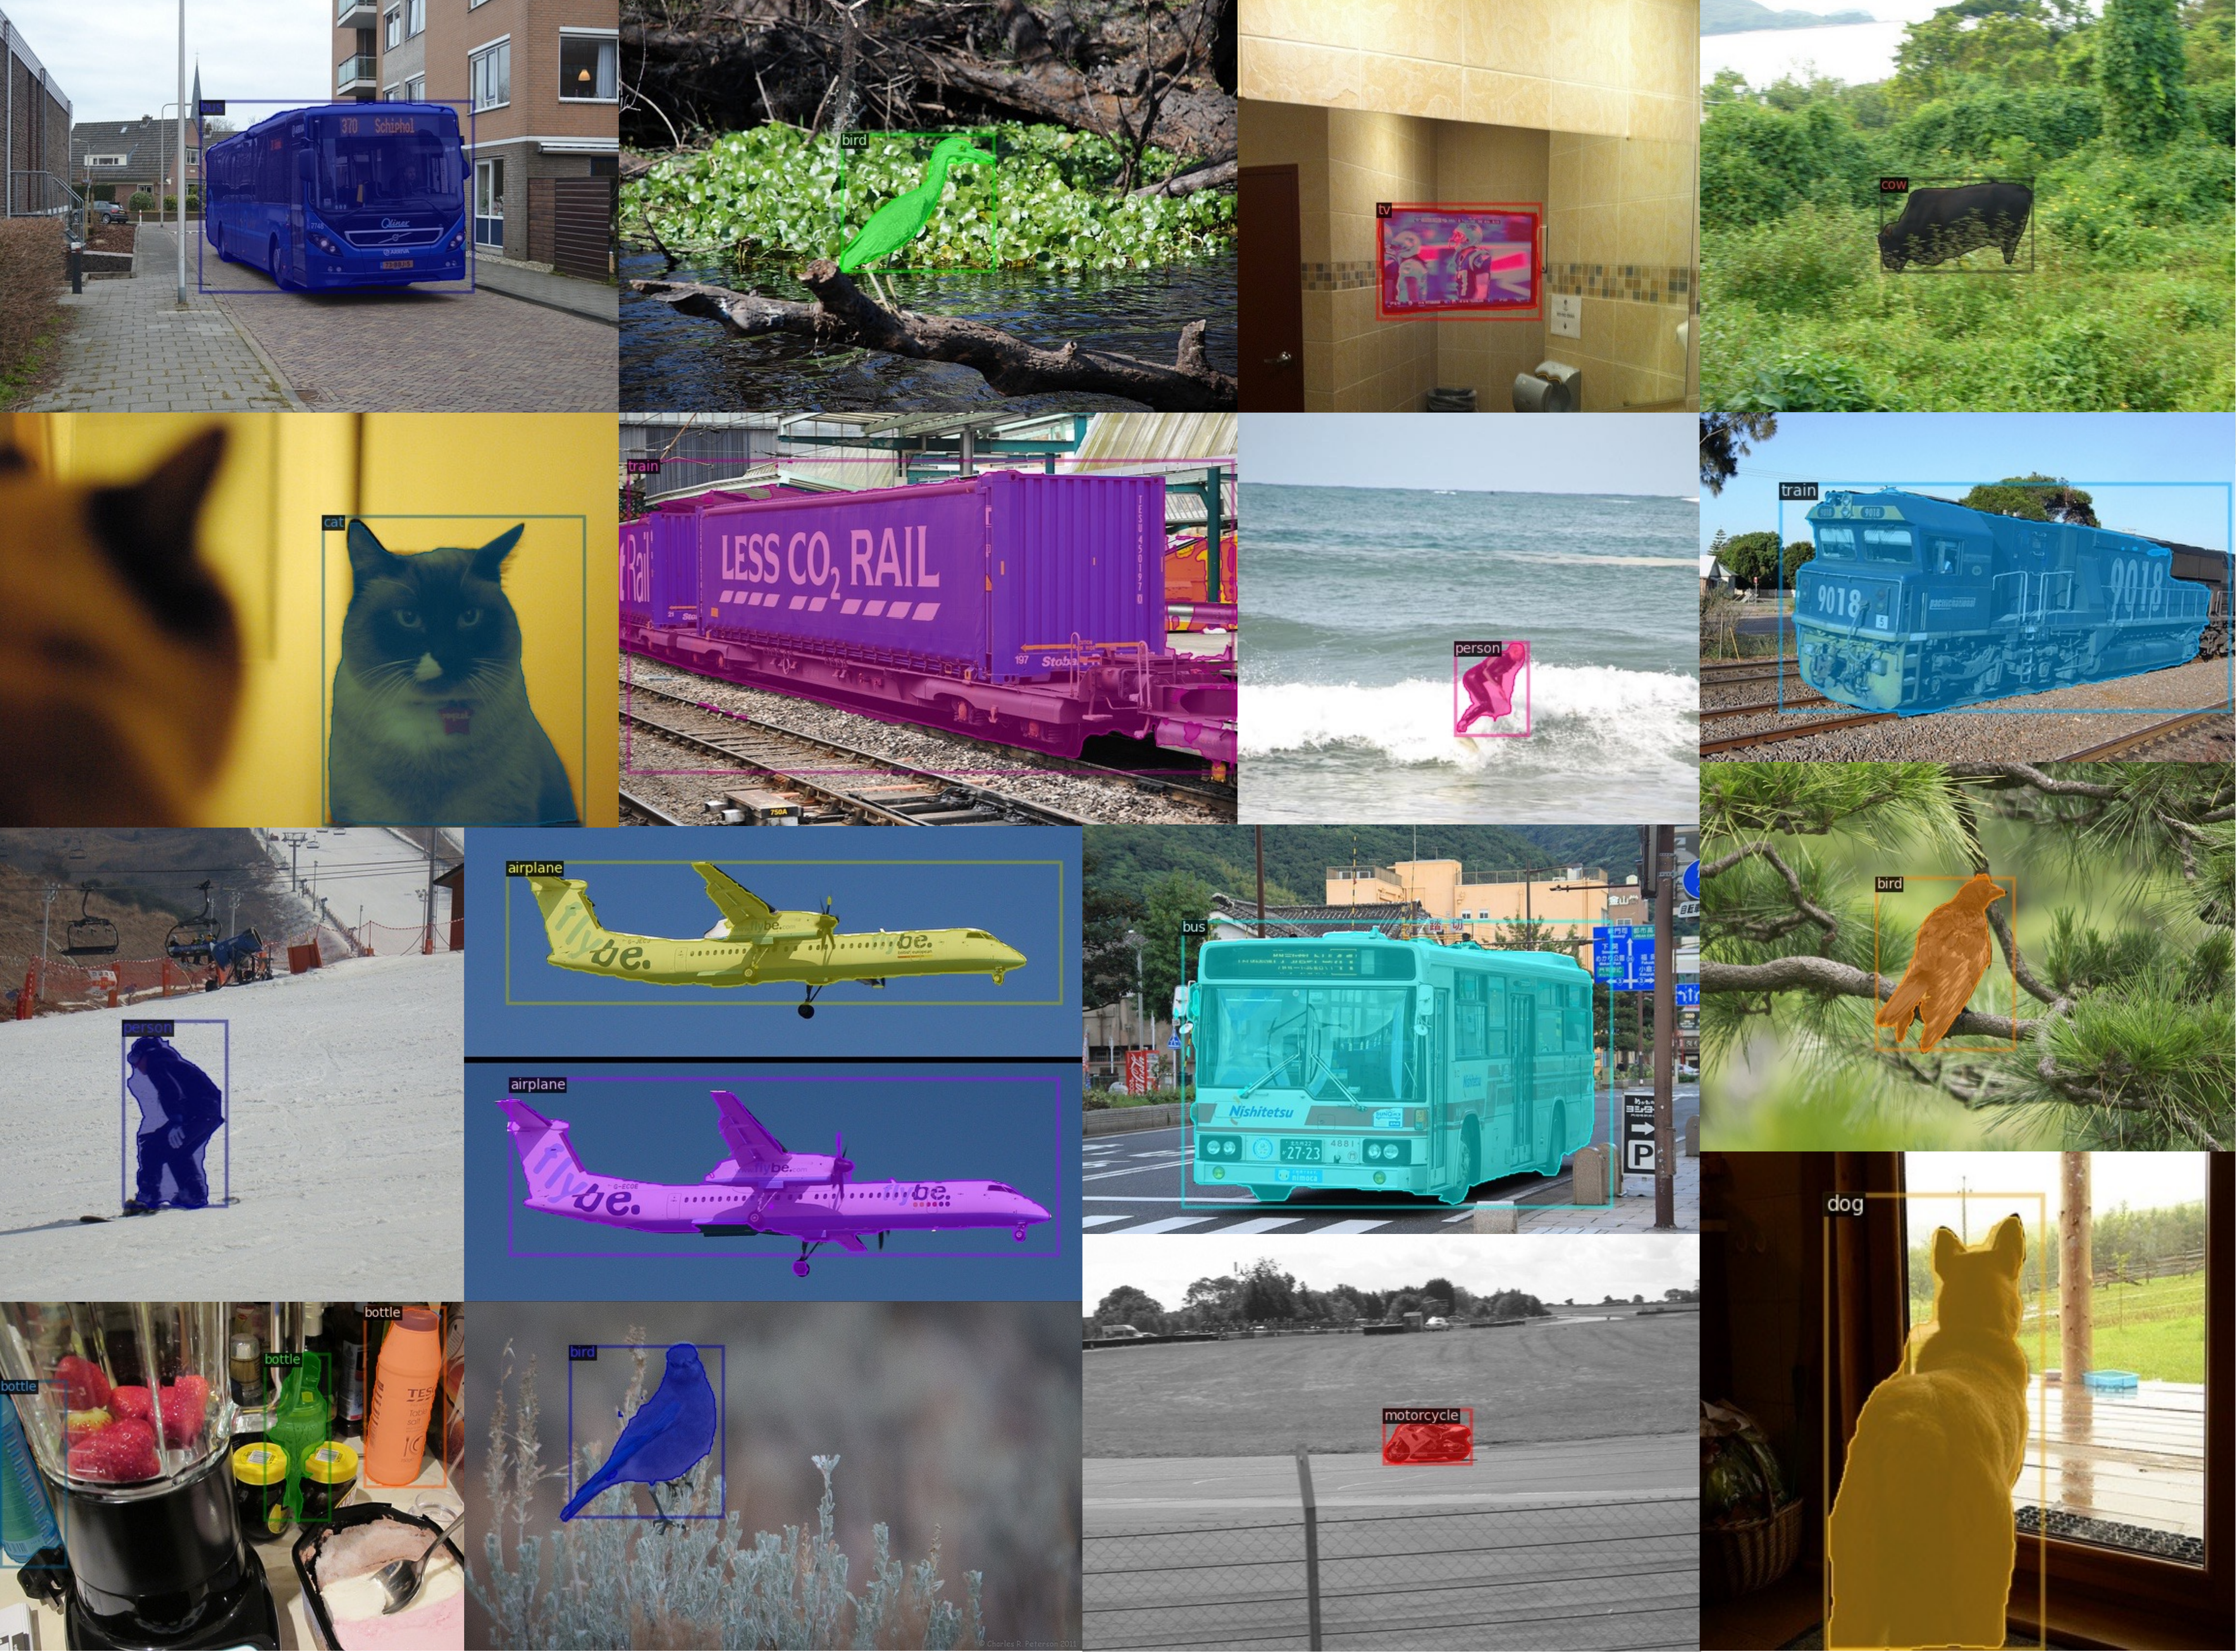}
    \caption{Additional qualitative results of ENInst for weakly-supervised low-shot instance segmentation on the MS-COCO dataset. The images with instances of different classes and sizes are segmented by only 10-shot weakly-labeled examples.}
    \label{fig:qualitative_coco_novel}
\end{figure*}

\begin{figure*}[t]
    \centering
    \includegraphics[width=1.0\linewidth,height=0.85\linewidth]{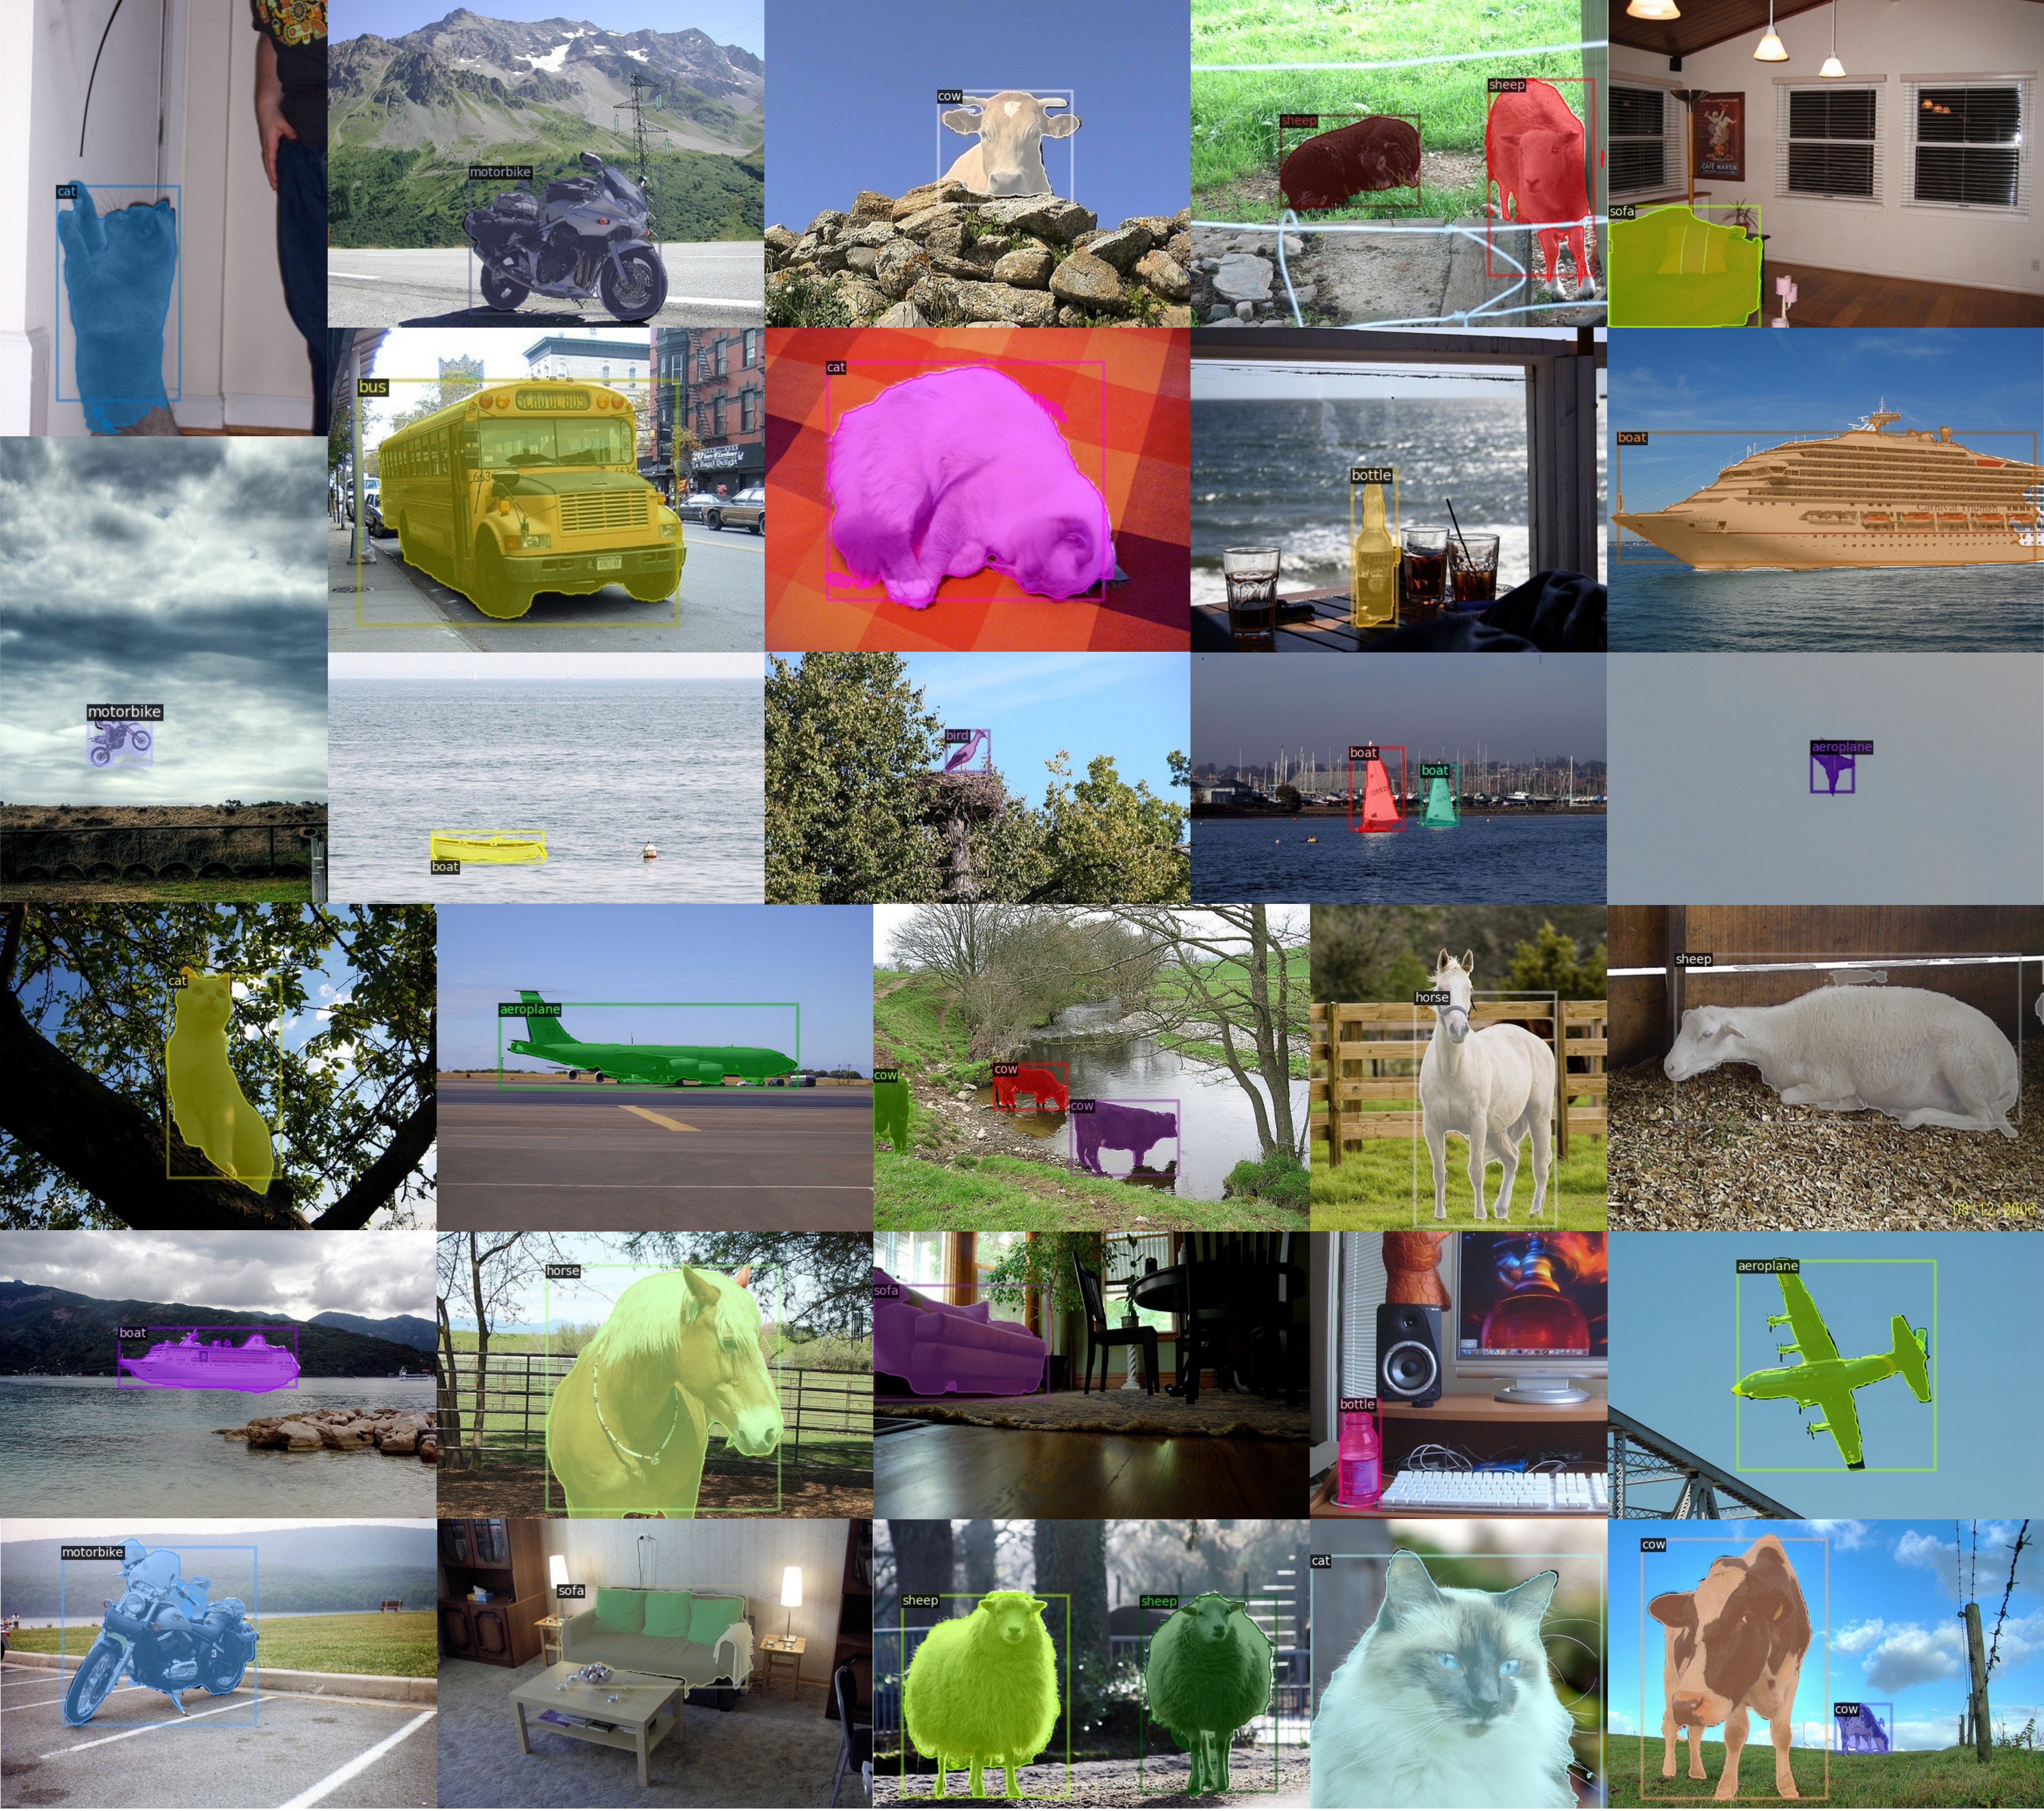}
    \caption{Qualitative results of our ENInst for weakly-supervised low-shot instance segmentation on the PASCAL VOC dataset. The images with instances of different classes and sizes are segmented by only 10-shot weakly-labeled examples.}
    \label{fig:qualitative_voc_novel}
\end{figure*}

\paragraph{VOC Novel}
We evaluate our method on PASCAL VOC and report the results of the three different split setups following Fan~\etal~\cite{fan2020fgn} in \Tref{tab:voc2voc_}.
The baseline consistently outperforms the GrabCut counterpart up to twice better in segmentation.
Our ENInst significantly increases the performance in both detection and segmentation tasks and thus achieves comparable performance to the fully-supervised MTFA.
In particular, our method shows better performance than MTFA for detection in Novel Class Setups 1 and 2, and even for the segmentation tasks in the 5 and 10-shot of Novel Class Setup 2.

% We summarize the implications of a few outperforming cases of our ENInst over the fully-supervised method, MTFA, as follows:
% \begin{itemize}
%     \item[$\bullet$] Despite the weak label, the small performance gap between MTFA and our ENInst in segmentation performance implies the effectiveness of our Instance-wise Mask Refinement (IMR) method.
%     \item[$\bullet$] It also implies that fast adaptation of our mask head in an optimization loop (feed-back, not a feed-forward) is the crucial design choice that can specialize to each instance.
%     \item[$\bullet$] 
%     % The classification components of our add-on modules, 
%     The enhancement method for classification accuracy, novel classifier composition (NCC),
%     % with Manifold Mixup,
%     % head fine-tuning, 
%     contributes to the outperforming cases in detection.
% \end{itemize}

We also present qualitative results of our ENInst on PASCAL VOC~\cite{everingham2010pascal} in \Fref{fig:qualitative_voc_novel}.
There are 5 classes in the query dataset of each setup.
There are some outstanding results that predict the masks even when the part of the instance is obscured ($1^{\mathrm{st}}$ row cow and sofa, $4^{\mathrm{th}}$ row cat ), the instance is very small ($2^{\mathrm{nd}}$ row motorbike, all of the images in $3^{\mathrm{rd}}$ row), and there are multiple instances ($3^{\mathrm{rd}}$ row boats, last row sheep and cows).

\begin{figure*}[t!]
     \centering
     \includegraphics[width=1.0\linewidth]{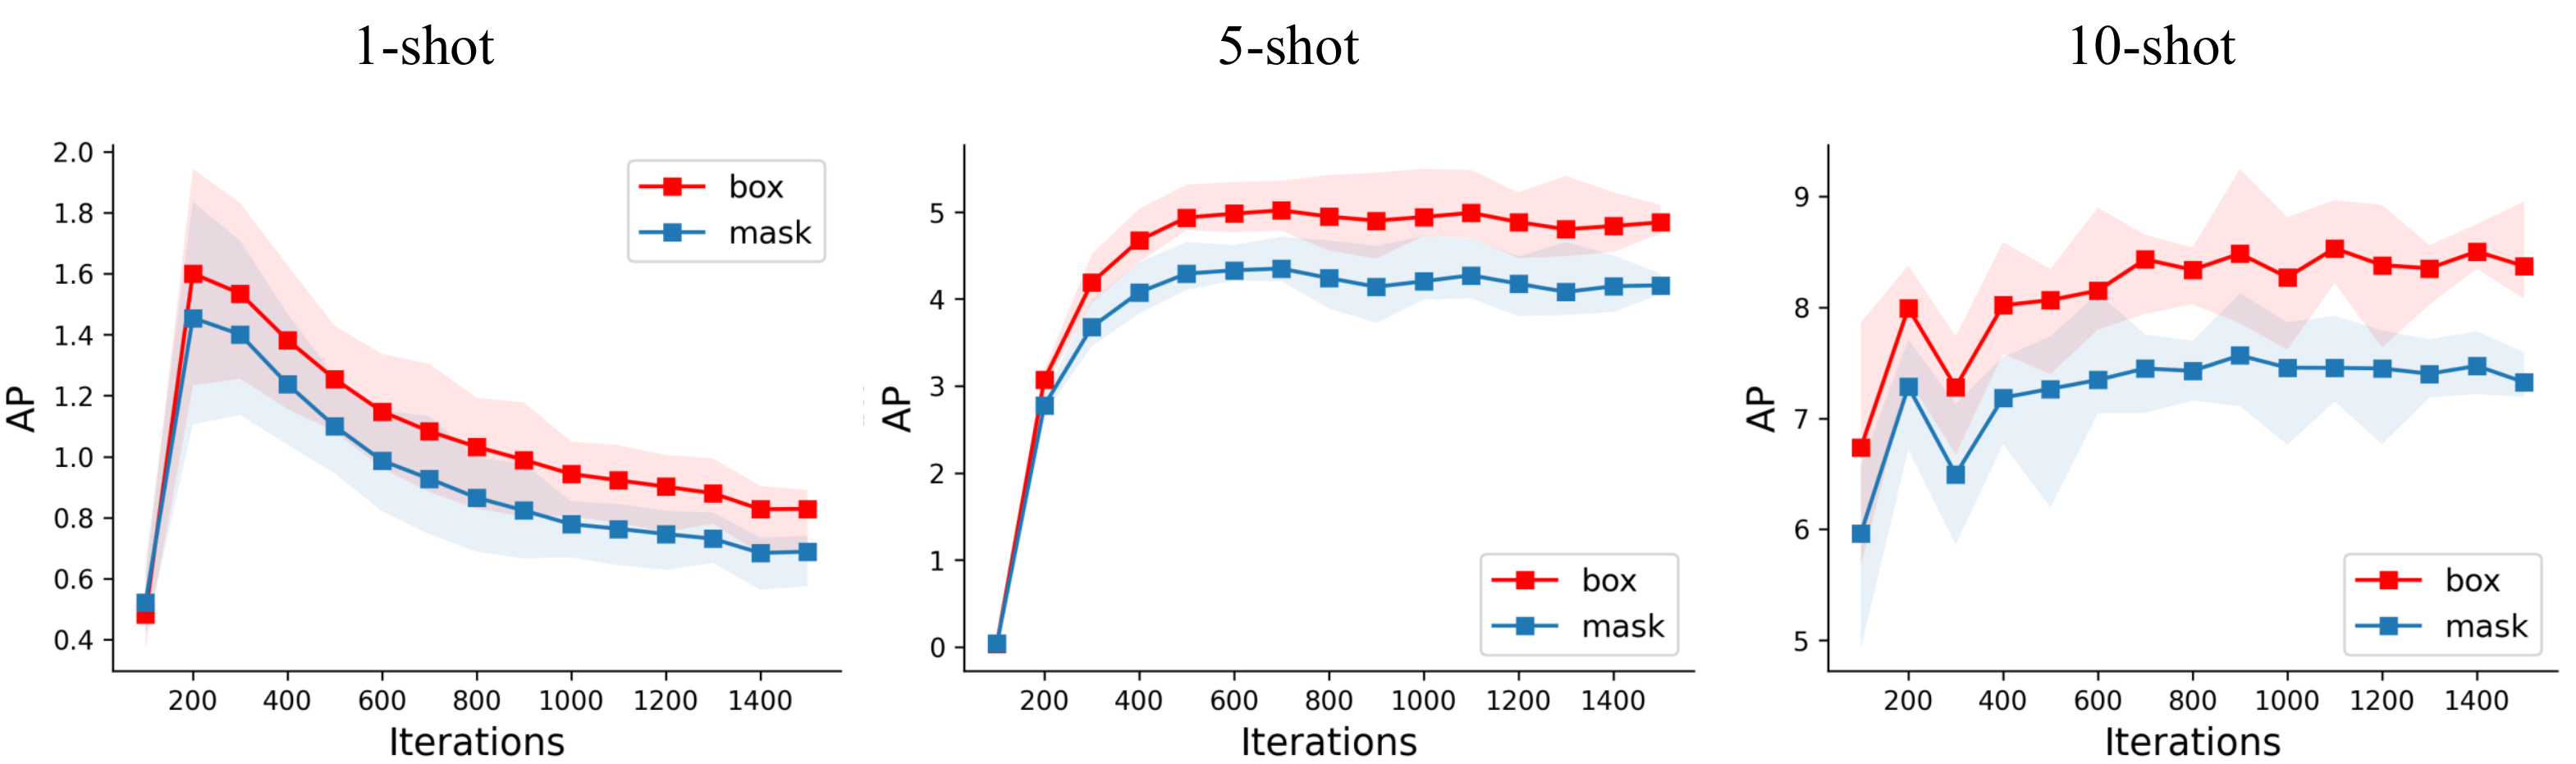}   
     \caption{Average precision according to the fine-tuning iterations.}
     \label{fig:iterations}
\end{figure*}

\subsection{Effects of Fine-tuning Iterations}\label{sec:C.2}
We conduct an experiment to see the effect of the number of iterations in the fine-tuning phase required for adaptation to the novel classes in \Fref{fig:iterations}.
We report the average performance of the baseline over 5 random trials according to the iterations with the COCO novel dataset.

In the 1-shot case, the model adapts quickly up to 200 iterations and then appears to be overfitting because the model is fine-tuned with only 20 images (20 classes with 1-shot sample per class).
From this empirical study, we set the fine-tuning iteration of the model to 200 in the 1-shot case to prevent overfitting, \ie, early termination strategy~\cite{zhang2021understanding}.
In the 5-shot case, the model is gradually trained, and the change after 800 iterations is negligible.
We set the iteration number to be 800 in the 5-shot setting in a similar spirit to the early termination so that we can prevent potential overfitting.
In the 10-shot case, the early iterations seem unstable, but the convergence is quickly stabilized later.
We hypothesize that this is because the capacity of the prediction heads is insufficient to deal with the diversity of 200 images (20 classes with 10-shot samples per class).
We set the 800 iterations in the 10-shot setting because the gain with additional iterations is negligible.
